# Supplementary material for: Finite-size effects on the Bose-Einstein condensation critical temperature in a harmonic trap
Source: arXiv:1603.07975 source file (2016-03-25)
Supplement: Supplementary file 1 [file supplementarymaterial.pdf]

# Supplementary material
for
Finite size effects on the Bose-Einstein condensation critical temperature

J.M.B. Noronha

*Universidade Lusíada - Porto, Rua Dr. Lopo de Carvalho, 4369-006 Porto, Portugal*

---

In the article, we defined the quantity $b_0$, which is related to the finite part at the $\alpha = 1$ pole of the 3-dimensional Barnes zeta function, $\zeta_B(\alpha, \epsilon|\boldsymbol{\lambda})$. It is dependent only on the anisotropy vector $\boldsymbol{\lambda}$. We present here a list of values of $b_0$ in the case of axially symmetric disc shaped and cigar shaped traps with integer aspect ratio $s$ between 1 and 100. Reasonable estimates of $b_0$ values for non-integer aspect ratios can be obtained from these by simple interpolation. Alternatively they can be computed from the exact expression in terms of an integral given in the article. Being $\omega_r$ and $\omega_z$ the radial and axial trap frequencies, we have $s = \omega_z/\omega_r$ for the disc shaped trap and $s = \omega_r/\omega_z$ for the cigar shaped trap.

Table 1: Values of $b_0$ for axially symmetric traps.

| Aspect ratio | Disc shape | Cigar shape |
|---:|---:|---:|
| 1 | -0.214451 | |
| 2 | 0.199078 | 0.243339 |
| 3 | 0.960542 | 1.131714 |
| 4 | 1.917153 | 2.244557 |
| 5 | 3.040325 | 3.517967 |
| 6 | 4.317999 | 4.918462 |
| 7 | 5.742927 | 6.424754 |
| 8 | 7.309997 | 8.021899 |
| 9 | 9.015311 | 9.698759 |
| 10 | 10.855751 | 11.446677 |
| 11 | 12.828756 | 13.258720 |
| 12 | 14.932171 | 15.129204 |
| 13 | 17.164161 | 17.053381 |
| 14 | 19.523137 | 19.027220 |
| 15 | 22.007714 | 21.047254 |

*Email address:* `jnoronha@por.ulusiada.pt` (J.M.B. Noronha)

*Preprint submitted to Physics Letters A* *July 3, 2015*

Table 1: (Continued).

| Aspect ratio | Disc shape | Cigar shape |
|---|---|---|
| 16 | 24.616664 | 23.110481 |
| 17 | 27.348907 | 25.214259 |
| 18 | 30.203467 | 27.356254 |
| 19 | 33.179474 | 29.534386 |
| 20 | 36.276128 | 31.746791 |
| 21 | 39.492717 | 33.991793 |
| 22 | 42.828585 | 36.267863 |
| 23 | 46.283126 | 38.573623 |
| 24 | 49.855785 | 40.907794 |
| 25 | 53.546060 | 43.269223 |
| 26 | 57.353459 | 45.656827 |
| 27 | 61.277563 | 48.069626 |
| 28 | 65.317952 | 50.506698 |
| 29 | 69.474244 | 52.967187 |
| 30 | 73.746079 | 55.450295 |
| 31 | 78.133130 | 57.955288 |
| 32 | 82.635069 | 60.481458 |
| 33 | 87.251620 | 63.028166 |
| 34 | 91.982483 | 65.594784 |
| 35 | 96.827394 | 68.180742 |
| 36 | 101.786129 | 70.785496 |
| 37 | 106.858424 | 73.408521 |
| 38 | 112.044062 | 76.049336 |
| 39 | 117.342833 | 78.707481 |
| 40 | 122.754521 | 81.382518 |
| 41 | 128.278963 | 84.074013 |
| 42 | 133.915950 | 86.781587 |
| 43 | 139.665309 | 89.504855 |
| 44 | 145.526865 | 92.243456 |
| 45 | 151.500477 | 94.997047 |
| 46 | 157.585981 | 97.765290 |
| 47 | 163.783223 | 100.547883 |
| 48 | 170.092068 | 103.344512 |
| 49 | 176.512404 | 106.154889 |
| 50 | 183.044042 | 108.978741 |
| 51 | 189.686912 | 111.815801 |
| 52 | 196.440866 | 114.665809 |
| 53 | 203.305776 | 117.528519 |
| 54 | 210.281580 | 120.403703 |
| 55 | 217.368121 | 123.291115 |
| 56 | 224.565314 | 126.190535 |
| 57 | 231.873027 | 129.101772 |

Table 1: (Continued).

| Aspect ratio | Disc shape | Cigar shape |
|---:|---:|---:|
| 58 | 239.291213 | 132.024591 |
| 59 | 246.819753 | 134.958823 |
| 60 | 254.458565 | 137.904254 |
| 61 | 262.207578 | 140.860707 |
| 62 | 270.066641 | 143.828003 |
| 63 | 278.035745 | 146.805973 |
| 64 | 286.114734 | 149.794441 |
| 65 | 294.303604 | 152.793250 |
| 66 | 302.602273 | 155.802227 |
| 67 | 311.010606 | 158.821249 |
| 68 | 319.528599 | 161.850136 |
| 69 | 328.156126 | 164.888769 |
| 70 | 336.893162 | 167.936989 |
| 71 | 345.739634 | 170.994653 |
| 72 | 354.695499 | 174.061667 |
| 73 | 363.760618 | 177.137861 |
| 74 | 372.935012 | 180.223132 |
| 75 | 382.218608 | 183.317363 |
| 76 | 391.611323 | 186.420404 |
| 77 | 401.113110 | 189.532176 |
| 78 | 410.723913 | 192.652550 |
| 79 | 420.443668 | 195.781418 |
| 80 | 430.272354 | 198.918673 |
| 81 | 440.209942 | 202.064207 |
| 82 | 450.256295 | 205.217918 |
| 83 | 460.411475 | 208.379722 |
| 84 | 470.675326 | 211.549500 |
| 85 | 481.047845 | 214.727170 |
| 86 | 491.529029 | 217.912655 |
| 87 | 502.118811 | 221.105820 |
| 88 | 512.817116 | 224.306629 |
| 89 | 523.623986 | 227.514969 |
| 90 | 534.539271 | 230.730747 |
| 91 | 545.562939 | 233.953893 |
| 92 | 556.695086 | 237.184337 |
| 93 | 567.935474 | 240.421971 |
| 94 | 579.284260 | 243.666748 |
| 95 | 590.741258 | 246.918582 |
| 96 | 602.306553 | 250.177387 |
| 97 | 613.980018 | 253.443125 |
| 98 | 625.761660 | 256.715687 |
| 99 | 637.651488 | 259.995015 |

Table 1: (Continued).

| Aspect ratio | Disc shape | Cigar shape |
|---|---|---|
| 100 | 649.649354 | 263.281048 |
